# Supplementary material for: IDEL: In-Database Entity Linking with Neural Embeddings
Source: arXiv:1803.04884 source file (2018-03-13)
Supplement: Supplementary file 1 [file appendix.tex]

\section*{Appendix I: IDEL SQL Queries}

\todoi{Show the whole workflow with generating embedding, create index, query index and using results of the query as code example}

\begin{lstlisting}[language=SQL, tabsize=2]
CREATE FUNCTION embed_sentence_for_building
  (sentences STRING)
RETURNS BLOB LANGUAGE PYTHON
{
  import monetdb_wrapper as mw
  data_repo = DataRepo("path/to/repo")
  encoder = \
    mw.encoder("path/to/model",data_repo)
  sentence_embedding = \
    encoder.encode_inputset2([sentences])
  return sentence_embedding
};
\end{lstlisting}

\begin{lstlisting}[language=SQL, tabsize=2]
CREATE TABLE sentences_with_embedding AS
SELECT *,
  embed_sentence_for_building(sentence)
    as embedding
FROM sentences;

CREATE TABLE building_with_embedding AS
SELECT *,
  embed_building(name, address, owner, ...)
    as embedding
FROM buildings;

CREATE TABLE similarity_building AS
SELECT
  s.key as skey, b.key ad bkey, *,
  similarity(s.embedding, b.embedding)
    AS sim
FROM
  sentences_with_embedding AS s,
  building_with_embedding AS b;
\end{lstlisting}

\begin{lstlisting}[language=SQL, tabsize=2]
CREATE VIEW rank_building AS
SELECT
  *,
  DENSE_RANK() over
    (PARTITION BY skey ORDER BY sim)
	AS rank
FROM similarity_building s;

SELECT * FROM rank_building
WHERE rank<10;
\end{lstlisting}

%\subsection*{Use case: Brand monitoring by matching product review with relational data and sentiment computation}
%\lstinputlisting[language=SQL, tabsize=2]{sqlexamples/sentiment.sql}
%\subsection*{Use case: Finding news which write about a supplier and products we order from them}
%\lstinputlisting[language=SQL, tabsize=2]{sqlexamples/relations.sql}
